# Supplementary material for: Bouncing Scenario and Cosmic Dynamics in Modified Theories of Gravity
Source: arXiv:2402.06895 source file (2024-02-10)
Supplement: Supplementary file 1 [file Appendices.tex]

% Appendix Template

\chapter{Appendices} % Main appendix title

\label{AppendixX} % Change X to a consecutive letter; for referencing this appendix elsewhere, use \ref{AppendixX}

\lhead{Appendix X. \emph{Appendix Title Here}} % Change X to a consecutive letter; this is for the header on each page - perhaps a shortened title
\textbf{Bianchi Type-III calculations}\\
For the line element (\ref{ch2met1}) the components of metric tensor $g_{\mu \nu}$ are\\

$g_{\mu \nu }=\left(
\begin{array}{cccc}
 1 & 0 & 0 & 0 \\
 0 & -A(t)^2 & 0 & 0 \\
 0 & 0 & -B(t)^2 & 0 \\
 0 & 0 & 0 & -B(t)^2 \\
\end{array}
\right)$
and 
$g^{\mu \nu }=\left(
\begin{array}{cccc}
 1 & 0 & 0 & 0 \\
 0 & -\frac{1}{A(t)^2} & 0 & 0 \\
 0 & 0 & -\frac{1}{B(t)^2} & 0 \\
 0 & 0 & 0 & -\frac{1}{B(t)^2} \\
\end{array}
\right)$\\

The non-vanishing Christoffel's symbols of the second kind for the line element (\ref{ch2met1}) are
\begin{eqnarray*}
 \text{$\Gamma$ [0, 1, 1]} = A(t) \dot{A}(t),   
 \text{$\Gamma$ [0, 2, 2]} = B(t) \dot{B}(t),  
 \text{$\Gamma$ [0, 3, 3]} = B(t) \dot{B}(t), \\
 \text{$\Gamma$ [1, 1, 0]} = \frac{\dot{A}(t)}{A(t)},  
 \text{$\Gamma$ [2, 2, 0]} = \frac{\dot{B}(t)}{B(t)},   
 \text{$\Gamma$ [3, 3, 0]} = \frac{\dot{B}(t)}{B(t)} 
\end{eqnarray*}
The non-vanishing components of $R_{\mu \nu}$ for the line element (\ref{ch2met1}) are

$\text{R[0, 0]} = -\frac{\ddot{A}(t)}{A(t)}-\frac{2 \ddot{B}(t)}{B(t)}$, $\text{R[1, 1]} = A(t) \left(\frac{2 \dot{A}(t) \dot{B}(t)}{B(t)}+\dot{A}(t)\right)$,\\
 $\text{R[2, 2]} = \dot{B}(t)^2+\frac{B(t) \dot{A}(t) \dot{B}(t)}{A(t)}+B(t) \dot{B}(t)$, $\text{R[3, 3]}= \dot{B}(t)^2+\frac{B(t) \dot{A}(t) \dot{B}(t)}{A(t)}+B(t) \dot{B}(t)$
%\begin{eqnarray*}
% \text{R[1, 1]} &=& -\frac{A''(t)}{A(t)}-\frac{2 B''(t)}{B(t)} \\
% \text{R[2, 2]} & A(t) \left(\frac{2 A'(t) B'(t)}{B(t)}+A''(t)\right) \\
% \text{R[3, 3]} & B'(t)^2+\frac{B(t) A'(t) B'(t)}{A(t)}+B(t) B''(t) \\
% \text{R[4, 4]} & B'(t)^2+\frac{B(t) A'(t) B'(t)}{A(t)}+B(t) B''(t) \\
%\end{eqnarray*}
