# Supplementary material for: Bouncing Scenario and Cosmic Dynamics in Modified Theories of Gravity
Source: arXiv:2402.06895 source file (2024-02-10)
Supplement: Supplementary file 2 [file AppendixA.tex]

% Appendix A
%\clearpage
\chapter{Appendix A} % Main appendix title

\label{AppendixA} % For referencing this appendix elsewhere, use \ref{AppendixA}

\lhead{Appendix \emph{Appendix A}} % This is for the header on each page - perhaps a shortened title

%%Write your Appendix content here.

$\left(
\begin{array}{cc}
 \text{$\Gamma $[1, 2, 2]} & A(t) A'(t) \\
 \text{$\Gamma $[1, 3, 3]} & B(t) B'(t) \\
 \text{$\Gamma $[1, 4, 4]} & B(t) B'(t) \\
 \text{$\Gamma $[2, 2, 1]} & \frac{A'(t)}{A(t)} \\
 \text{$\Gamma $[3, 3, 1]} & \frac{B'(t)}{B(t)} \\
 \text{$\Gamma $[4, 4, 1]} & \frac{B'(t)}{B(t)} \\
\end{array}
\right)$
